# Supplementary material for: Transform Once: Efficient Operator Learning in Frequency Domain
Source: arXiv:2211.14453 source file (2022-11-26)
Supplement: Supplementary file 1 [file _appendix_dev.tex]

\documentclass{article}
\usepackage[nonatbib]{neurips_2022}
\input{template/style}
\input{template/math}
\input{config}

\begin{document}

%%%% APPENDIX %%%%%
\input{sections/appendix/_main}

\end{document}
